# Supplementary material for: Methylbenzenes on graphene
Source: arXiv:1607.05107 ancillary file (2016-07-18)
Supplement: Supplementary file 1 [file BTXM_adsorption_data_vdW-DF1.pdf]

# Supplementary material for

# «Methylbenzenes on graphene»

Øyvind Borck
*Randaberg videregående skole, Grødemveien 70, NO-4070 Randaberg, Norway*

Elsebeth Schröder
*Microtechnology and Nanoscience, MC2, Chalmers University of Technology, SE-412 96 Göteborg, Sweden*

Adsorption energies and configurations of methylbenzenes on graphene computed using density functional theory with the vdW-DF1 method [1]. For each methylbenzene we present all the considered positions of the molecule on graphene, in the following order: Benzene, toluene, para-xylene (p-xylene), meta-xylene (m-xylene), ortho-xylene (o-xylene), and mesitylene. 'Top', 'bridge' and 'hollow' refers to the position of the center of the aromatic ring with respect to graphene. 'Edge' refers to configurations where the methyl group is oriented with two of the H atoms closer to the graphene than the methyl group C atom, while 'corner' refers to configurations where only one H atom is closer to graphene than the C atom. Different configurations can be obtained by rotating the molecules around the center of the aromatic ring. 'Rotated' indicates how many degrees the molecule has been rotated with respect to a reference configuration (rotated $0^{o}$).

[1] M. Dion, H. Rydberg, E. Schröder, D. C. Langreth, and B. I Lundqvist, Phys. Rev. Lett. 92, 246401 (2004); 109902 (E) (2005).

# Benzene

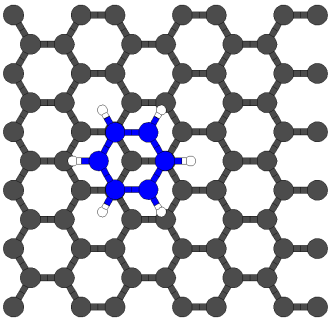

429.81 meV
Top site.

# Toluene

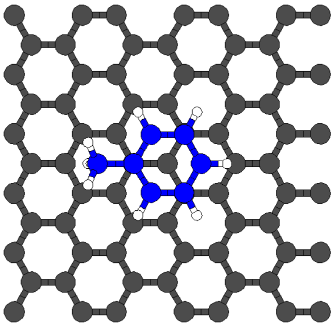

498.37 meV
Top, corner, rotated 0°.

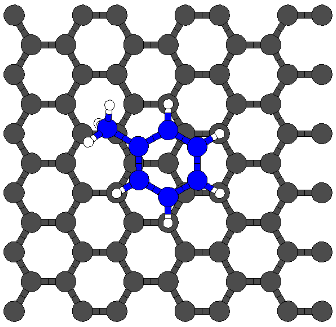

493.65 meV
Top, corner, rotated 30°.

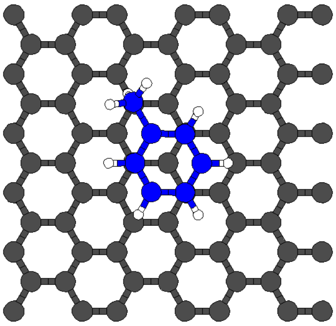

492.66 meV
Top, corner, rotated 60°.

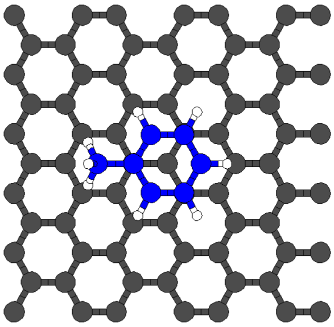

520.52 meV
Top, edge, rotated 0°.

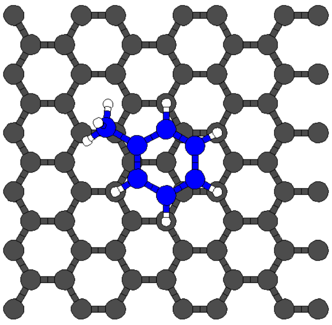

520.95 meV
Top, edge, rotated 30°.

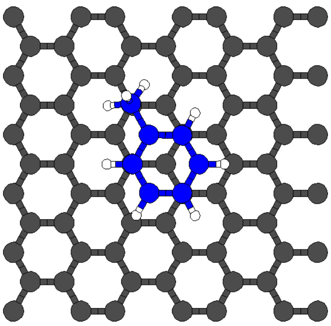

521.00 meV
Top, edge, rotated 60°.

# Toluene

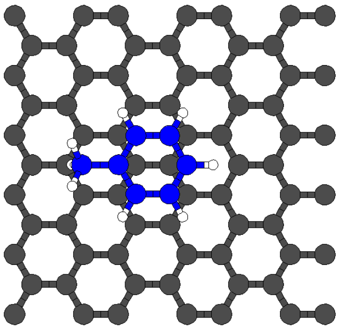

495.97 meV
Bridge, corner, rotated $0^o$.

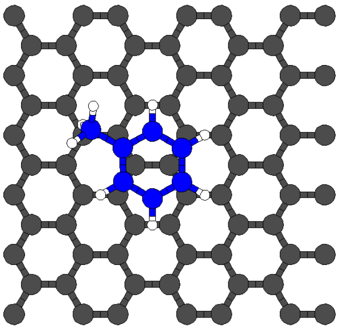

491.74 meV
Bridge, corner, rotated $30^o$.

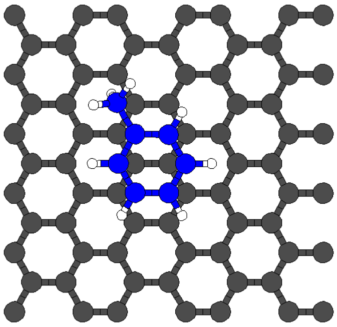

488.43 meV
Bridge, corner, rotated $60^o$.

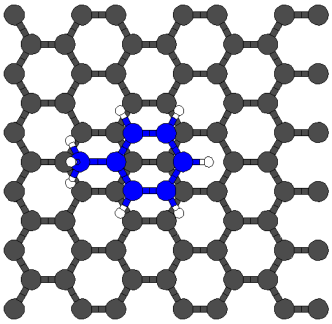

520.31 meV
Bridge, edge, rotated $0^o$.

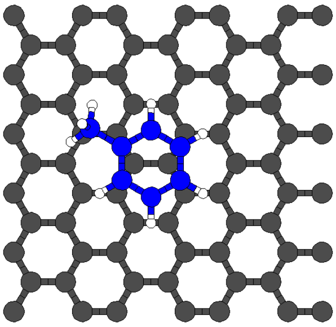

518.69 meV
Bridge, edge, rotated $30^o$.

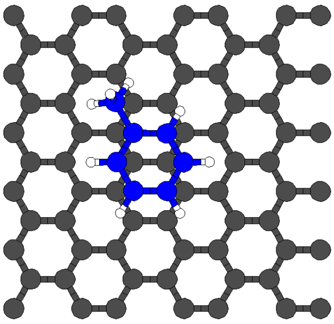

515.81 meV
Bridge, edge, rotated $60^o$.

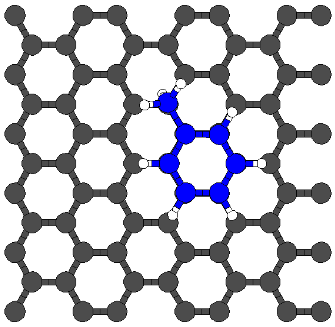

475.62 meV
Hollow, corner, rotated $0^o$.

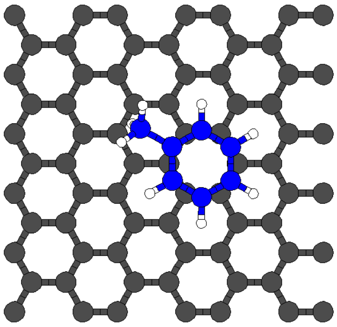

477.82 meV
Hollow, corner, rotated $30^o$.

# Toluene

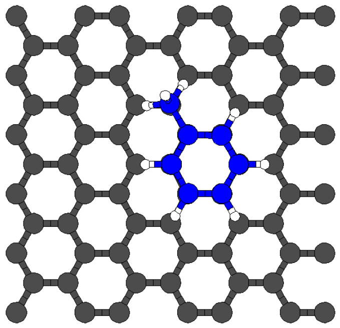

503.51 meV
Hollow, edge, rotated 0°.

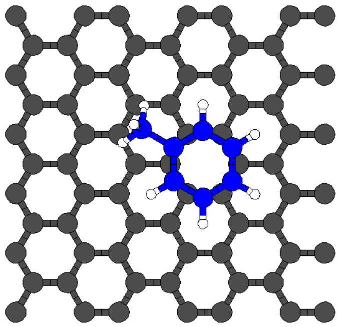

503.87 meV
Hollow, edge, rotated 30°.

# p-Xylene

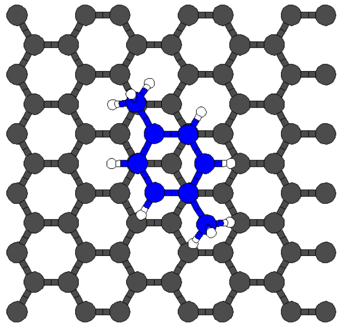

610.43 meV
Top, edge, rotated 0°.

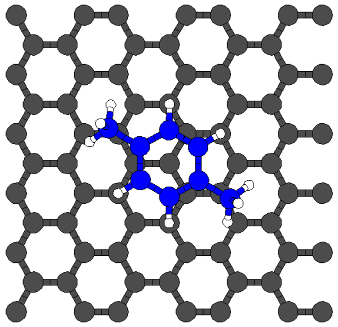

610.28 meV
Top, edge, rotated 30°.

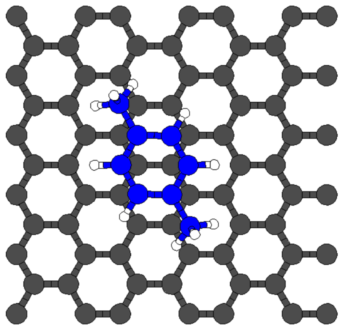

610.74 meV
Bridge, edge, rotated 0°.

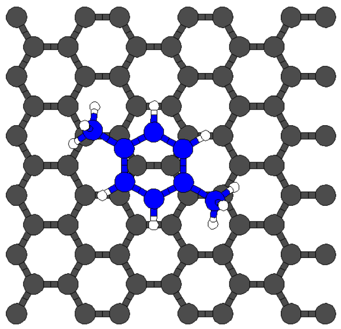

607.39 meV
Bridge, edge, rotated 30°.

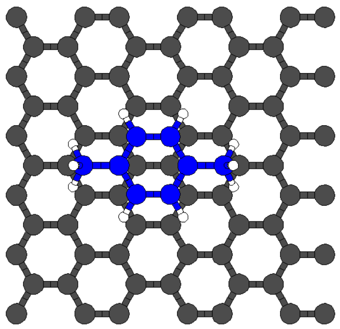

602.04 meV
Bridge, edge, rotated 60°.

## p-Xylene

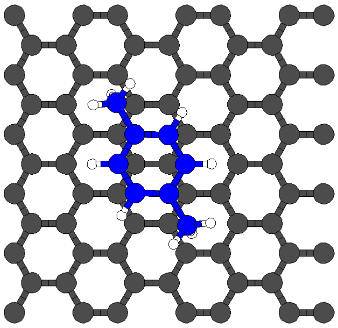

556.58 meV
Bridge, corner, rotated $0^{o}$.

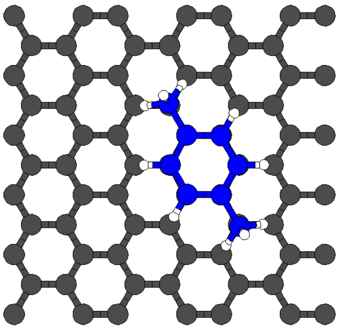

589.13 meV
Hollow, edge, rotated $0^{o}$.

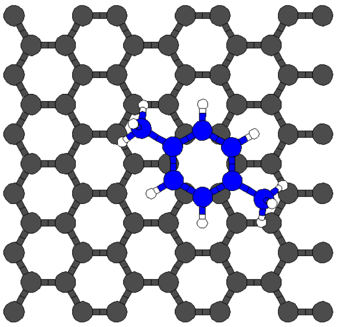

589.58 meV
Hollow, edge, rotated $30^{o}$.

## m-Xylene

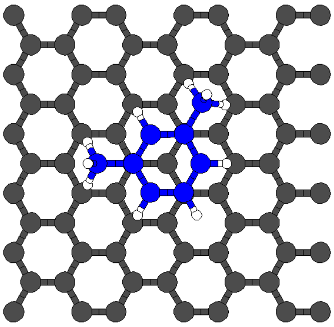

611.07 meV
Top, edge, rotated $0^{o}$.

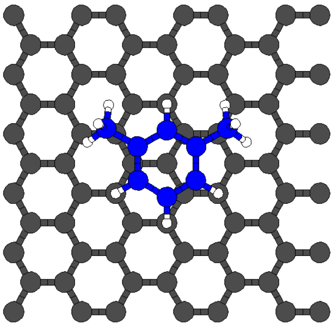

612.36 meV
Top, edge, rotated $30^{o}$.

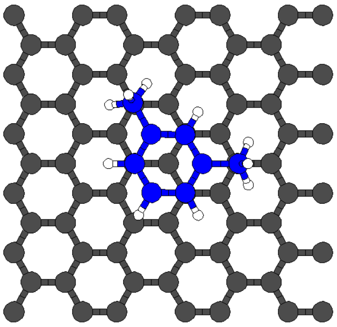

610.55 meV
Top, edge, rotated $60^{o}$.

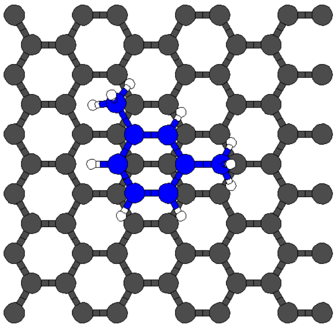

606.82 meV
Bridge, edge, rotated $0^{o}$.

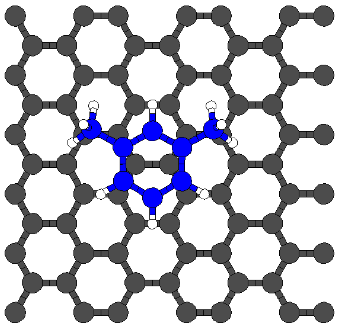

609.19 meV
Bridge, edge, rotated $30^{o}$.

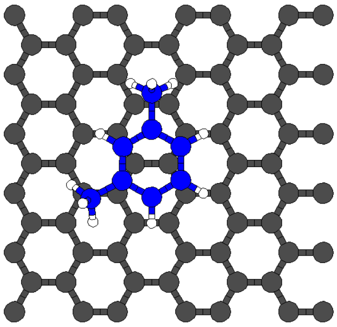

609.47 meV
Bridge, edge, rotated $90^{o}$.

# m-Xylene

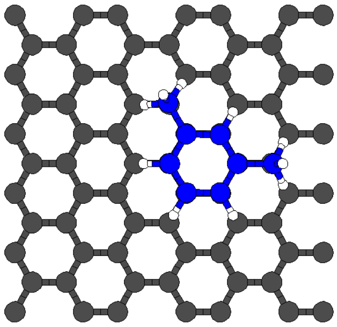

586.60 meV
Hollow, edge, rotated 0°.

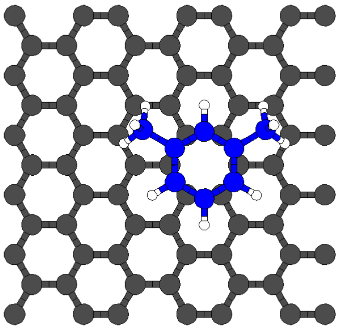

589.02 meV
Hollow, edge, rotated 30°.

# o-Xylene

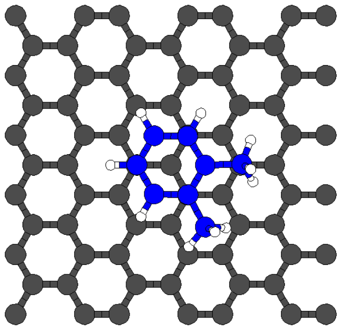

588.70 meV
Top, edge, rotated 0°.

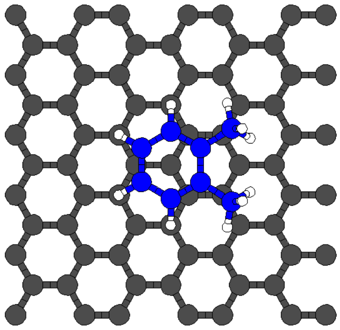

588.71 meV
Top, edge, rotated 30°.

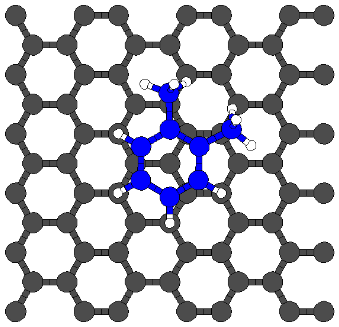

586.91 meV
Top, edge, rotated 90°.

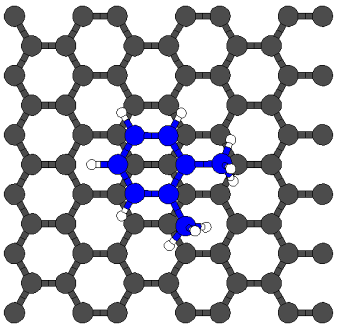

581.91 meV
Bridge, corner, rotated 0°.

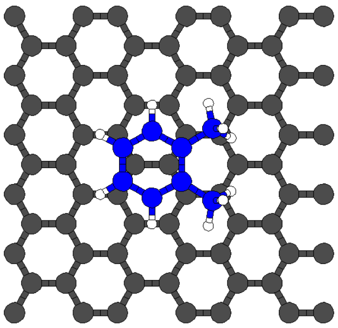

587.46 meV
Bridge, corner, rotated 30°.

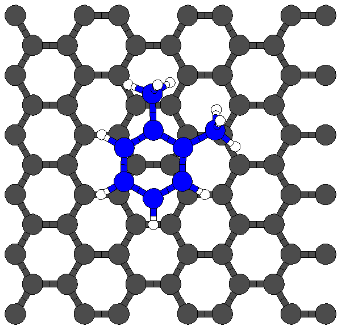

581.91 meV
Bridge, corner, rotated 90°.

## o-Xylene

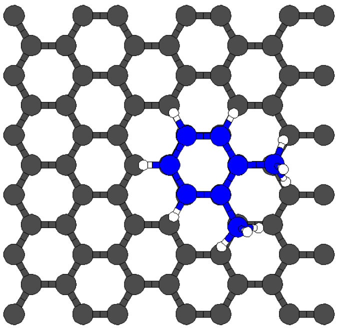

564.72 meV
Hollow, edge, rotated 0°.

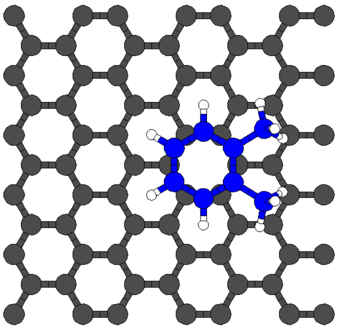

565.67 meV
Hollow, edge, rotated 30°.

## Mesitylene

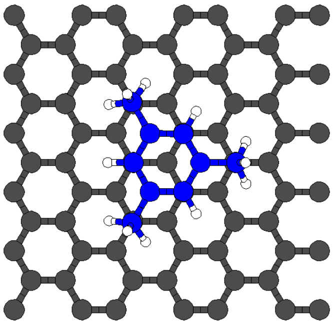

699.44 meV
Top, edge, rotated 0°.

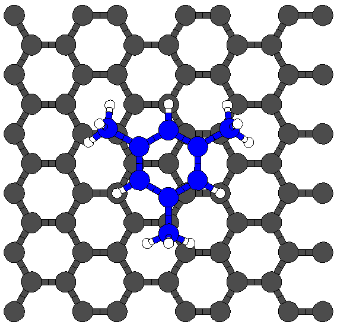

700.26 meV
Top, edge, rotated 30°.

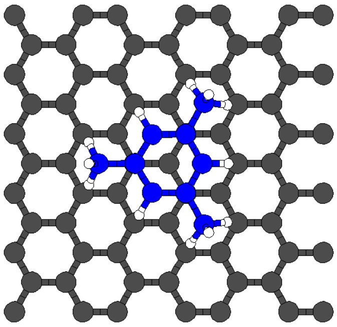

700.56 meV
Top, edge, rotated 60°.

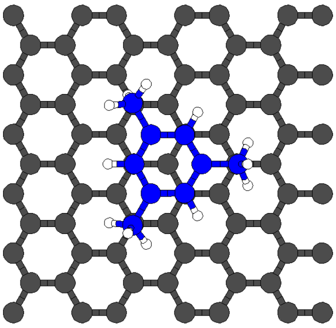

670.87 meV
Top, one corner, two edge, rotated 0°.

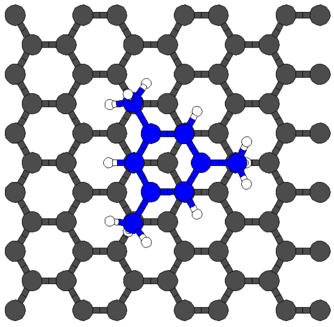

638.75 meV
Top, two corner, one edge, rotated 0°.

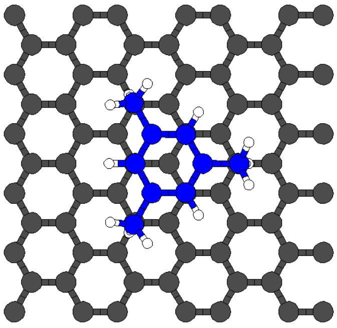

602.01 meV
Top, edge, rotated 0°.

# Mesitylene

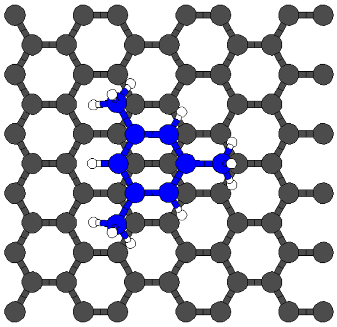

697.57 meV
Bridge, edge, rotated $0^o$.

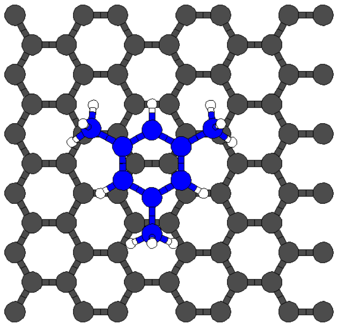

697.66 meV
Bridge, edge, rotated $30^o$.

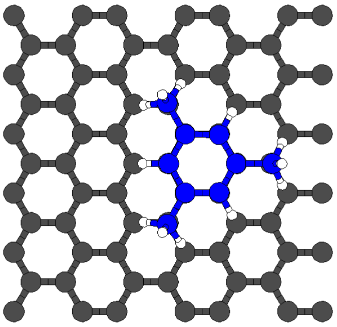

637.36 meV
Hollow, edge, rotated $0^o$.

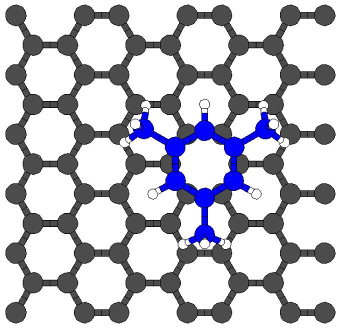

676.60 meV
Hollow, edge, rotated $30^o$.
